# Supplementary material for: Deep Decomposition for Stochastic Normal-Abnormal Transport
Source: arXiv:2111.14777 source file (2022-03-28)
Supplement: Supplementary file 2 [file app_2d_demo.tex]

\section{Simulation: Anisotropic Flying Points}
\label{app: 2d_demo}
