# Supplementary material for: Deep Decomposition for Stochastic Normal-Abnormal Transport
Source: arXiv:2111.14777 source file (2022-03-28)
Supplement: Supplementary file 7 [file exp_setting.tex]

\section{Experimental Settings and Details}
\label{app: settings}
