# Supplementary material for: Deep Decomposition for Stochastic Normal-Abnormal Transport
Source: arXiv:2111.14777 source file (2022-03-28)
Supplement: Supplementary file 10 [file main_empty.tex]

\clearpage
\onecolumn
\appendix

{\centering 
\section*{Deep Decomposition for Stochastic Normal-Abnormal Transport\\Supplementary Material}
}

%%%%%%%%%%%%%%%%%%%%%%%%%%%%%%%

\section{Theorem 1: Divergence-free Vector Representation by the Curl of Potentials}
\label{app: proof_div_free}

\section{Theorem 2: Symmetric PSD Tensor Representation by Spectral Decomposition}
\label{app: proof_psd}

\section{PyTorch PDE Solver: Numerical Derivations and Software Descriptions}
\label{app: numericals}

\section{Simulative Brain Advection-Diffusion Dataset}
\label{app: ixi}

%\section{Additional Experimental Results}
%\label{app: results}

%\section{Mathematical Preliminaries}
%\label{sec: preliminaries}
